# Supplementary material for: Point Primitive Transformer for Long-Term 4D Point Cloud Video Understanding
Source: arXiv:2208.00281 source file (2022-12-20)
Supplement: Supplementary file 2 [file supp.tex]

\setcounter{section}{0}

This document provides a list of supplemental materials to support the main paper.
\begin{itemize}
    % \item \textbf{Primitive v.s. Supervoxel} - To further demonstrate the power of primitive representation, we compare our method with supervoxel-based transformer.
    \item \textbf{Does primitive play the role of label smoothing?} - We conduct experiments to explore if primitive play the role of label smoothing.
    \item \textbf{Curves of Training process and Occupied memory.} - We provide training and memory-clip curves to verify the efficiency of our more optimization friendly PPTr.
    \item \textbf{Visualization} - We provide some visualization results of 4D semantic segmentation and primitive fitting.
\end{itemize}

% \section{Primitive v.s. Supervoxel}
% \label{sec:Supervoxel}
% We propose to construct a point primitive transformer using primitive as an intermediate representation. In order to further prove the power of primitive, we replace primitive with supervoxel as the basis for space division and conduct experiments on sythia4D. We find that PPTr with supervoxel results in a $3.79\%$ mIoU drop, which demonstrates the importance of leveraging the primitive plane to capture the long-term spatial-temporal context.
\section{Does primitive play the role of label smoothing?}
\label{sec:smoothing}
We conducted experiments on Sythia4D to determine if the primitive plays the role of label smoothing. We directly vote the label with the most as the primitive label, then calculate mIoU. However, we can only achieve 44.59 mIoU in this way, which shows that simple label smoothing is not sufficient to achieve better performance. This also proves that primitive does not play the role of label smoothing, but acts as an intermediate representation to capture long-term spatio-temporal information more effectively.

\section{Curves of Training process and Occupied memory.}
 To verify the model efficiency and whether our PPTr reduces the optimization difficulty of the transformer, we provide the network training curve along with a memory growth curve as the clip length increases in figure~\ref{fig:curve}. Our model can quickly reach accuracy above 35, while P4Transformer can only reach about 5 when getting only one epoch trained. The results also show that our model reduces the memory requirements for training significantly when clip length is relatively long.
 \begin{figure}[htbp]
    \centering
    \includegraphics[width=9cm]{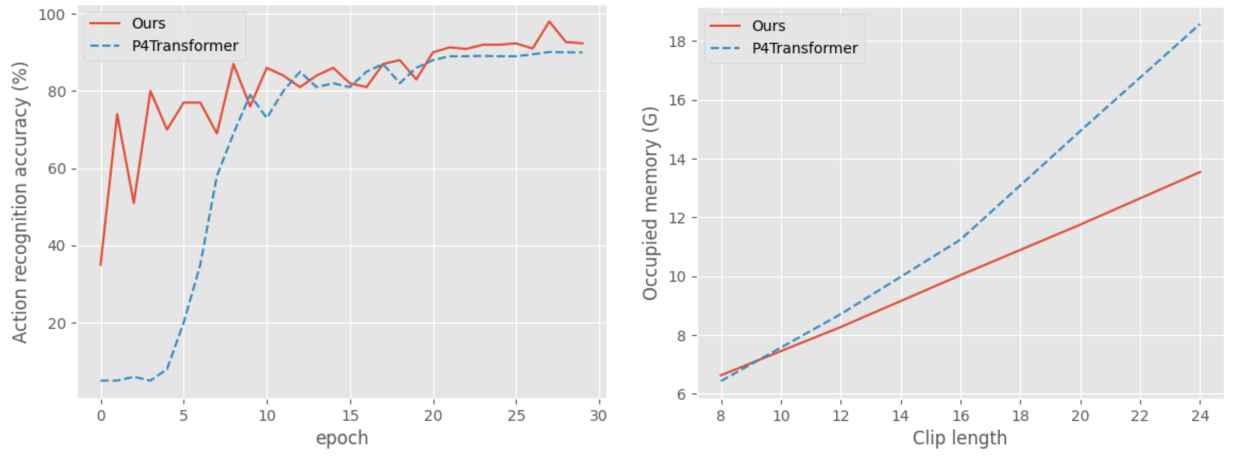}
    \caption{Curve of Training process and Occupied memory.}
    \label{fig:curve}
\end{figure}
\section{Visualization}
\label{sec:Visualization}
We provide visualizations of HOI4D 4D semantic segmentation and some primitive fitting results in figure~\ref{fig:suppvis}.
\begin{figure}[t]
    \centering
    \includegraphics[width=10cm]{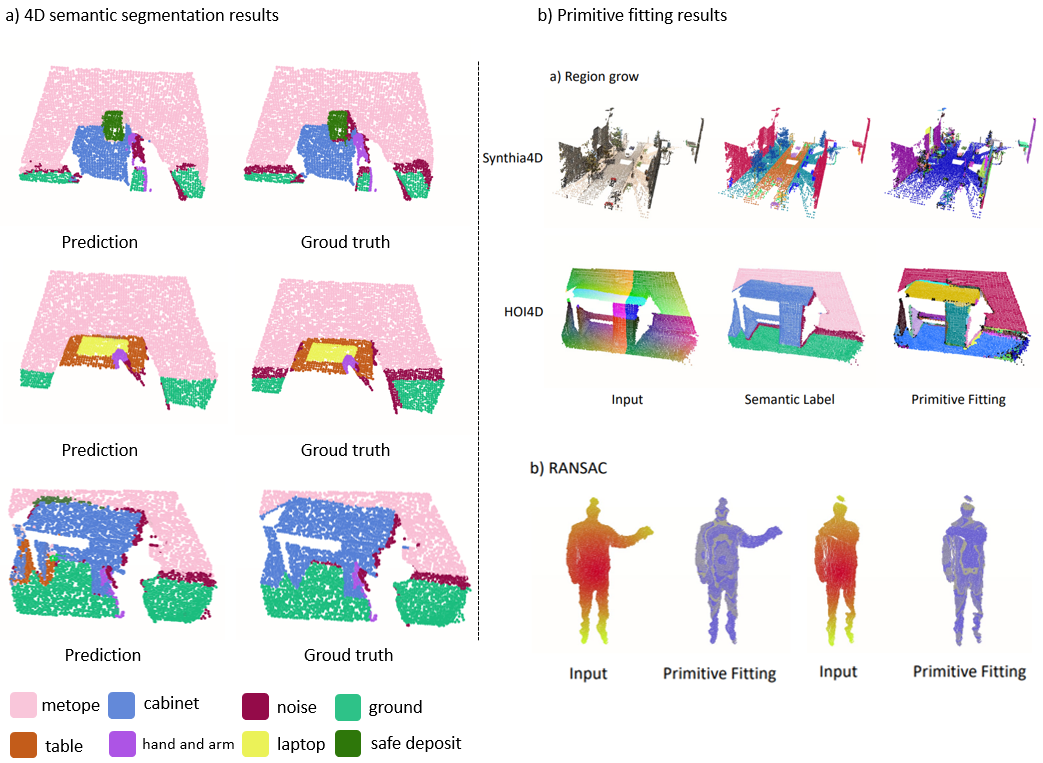}
    \caption{Visualizations of HOI4D 4D semantic segmentation and some primitive fitting results}
    \label{fig:suppvis}
    % \vspace{-20pt}
\end{figure}
